# Supplementary material for: There and Back Again: Learning to Simulate Radar Data for Real-World Applications
Source: arXiv:2011.14389 source file (2020-11-29)
Supplement: Supplementary file 1 [file 6-appendix.tex]

\section{Appendix}
\begin{table}[h]
    \centering
    \begin{tabular}{cccc}
    \toprule
    Dataset & Domain & Mode & N \\
    \midrule
     $\mathbb{R}$ & Real   & Train &  $222420$   \\
     $\mathbb{T}$ & Real & Test & $23460$ \\
     $\mathbb{S}$ & Simulation & Train & $100000$ \\
     $\mathbb{C}$ & Simulation & Test & $68400$  \\
    \bottomrule
    \end{tabular}
    \vspace{0.5em}
    \caption{An overview of the datasets used in the experiments.}
    \label{tab:datsets}
\end{table}
